# Supplementary material for: Exploring Magnetism of Lead-free Halide Double Perovskites: A High-Throughput First-Principles Study
Source: arXiv:2306.09300 source file (2023-06-15)
Supplement: Supplementary file 1 [file SI.pdf]

# Exploring Magnetism of Lead-free Halide Double Perovskites: A High-Throughput First-Principles Study

Utkarsh Singh,[1,*] Johan Klarbring,[1] Igor A. Abrikosov,[1] and Sergei I. Simak[1,2]

[1] *Theoretical Physics Division, Department of Physics, Chemistry and Biology (IFM), Linköping University, SE-581 83, Linköping, Sweden*

[2] *Department of Physics and Astronomy, Uppsala University, SE-75120 Uppsala, Sweden*

(Dated: June 15, 2023)

* utkarsh.singh[at]liu.se

TABLE S1. List of (Column 1) screened $Cs_2BB'Cl_6$ LFHDPs and corresponding (Column 2) modified tolerance factor, $\tau$, (Column 3) distance to convex hull for the cubic ferromagnetic double perovskite phase from previous studies, $\Delta H_{hull}$. The subsequent columns specify the conducting nature, magnetic configuration, and distortion from the cubic phase (c/a) respectively of calculated magnetic ground state determined in this work.

| $A_2BB'Cl_6$ | $\tau$ | **$\Delta H_{hull}$ (cubic ferromagnetic phase)** | **Metal / Insulator (Ground state)** | **Calculated magnetic ground state** | **c/a** | **Calculated magnetic moments, B/B' $\in$ 3d$^{1-9}$** |
|---|---|---|---|---|---|---|
| $Cs_2NaTiCl_6$ | 0.65 | 0.000 | Metal | FM | 0.991 | –, 0.903 |
| $Cs_2NaVCl_6$ | 0.64 | 0.000 | Metal | AFM-3 | 0.992 | –, 1.918 |
| $Cs_2NaMnCl_6$ | 0.64 | 0.000 | Metal | FM | 1.000 | –, 4.035 |
| $Cs_2NaFeCl_6$ | 0.64 | 0.000 | Insulator | AFM-1 | 0.996 | –, 4.053 |
| $Cs_2NaNiCl_6$ | 0.62 | 0.025 | Metal | FM | 1.000 | –, 1.000 |
| $Cs_2KTiCl_6$ | 0.71 | 0.000 | Metal | FM | 1.002 | –, 0.894 |
| $Cs_2KVCl_6$ | 0.71 | 0.000 | Metal | FM | 1.010 | –, 1.982 |
| $Cs_2KCrCl_6$ | 0.71 | 0.000 | Insulator | AFM-1 | 1.000 | –, 2.995 |
| $Cs_2KMnCl_6$ | 0.71 | 0.000 | Metal | AFM-1 | 1.049 | –, 4.014 |
| $Cs_2KFeCl_6$ | 0.71 | 0.009 | Insulator | AFM-1 | 0.996 | –, 4.004 |
| $Cs_2KNiCl_6$ | 0.71 | 0.028 | Metal | AFM-1 | 1.044 | –, 1.014 |
| $Cs_2AgMnCl_6$ | 0.69 | 0.031 | Metal | FM | 1.000 | –, 4.001 |
| $Cs_2AgNiCl_6$ | 0.67 | 0.000 | Metal | FM | 1.025 | –, 1.276 |
| $Cs_2AgTiCl_6$ | 0.69 | 0.000 | Metal | AFM-1 | 0.998 | –, 0.909 |
| $Cs_2AgFeCl_6$ | 0.69 | 0.000 | Insulator | AFM-1 | 0.983 | –, 3.974 |
| $Cs_2AgVCl_6$ | 0.68 | 0.000 | Metal | AFM-1 | 0.997 | –, 1.951 |
| $Cs_2AgCoCl_6$ | 0.68 | 0.000 | Metal | AFM-3 | 0.990 | –, 2.501 |
| $Cs_2AuVCl_6$ | 0.71 | 0.000 | Insulator | FM | 0.896 | –, 2.021 |
| $Cs_2AuCrCl_6$ | 0.71 | 0.000 | Metal | AFM-1 | 0.926 | –, 3.214 |
| $Cs_2AuMnCl_6$ | 0.71 | 0.000 | Metal | FM | 1.000 | –, 4.349 |
| $Cs_2AuFeCl_6$ | 0.71 | 0.000 | Insulator | AFM-1 | 0.934 | –, 3.887 |
| $Cs_2AuCoCl_6$ | 0.71 | 0.000 | Metal | AFM-1 | 1.105 | –, 2.368 |
| $Cs_2AuNiCl_6$ | 0.71 | 0.009 | Metal | FM | 1.098 | –, 1.265 |
| $Cs_2CaTiCl_6$ | 0.7 | 0.000 | Metal | FM | 1.004 | –, 1.638 |
| $Cs_2CaVCl_6$ | 0.68 | 0.000 | Insulator | AFM-3 | 1.001 | –, 2.671 |
| $Cs_2CaCrCl_6$ | 0.69 | 0.000 | Metal | AFM-1 | 1.052 | –, 3.733 |
| $Cs_2CaMnCl_6$ | 0.69 | 0.000 | Metal | AFM-3 | 1.000 | –, 4.557 |
| $Cs_2SnVCl_6$ | 0.71 | 0.039 | Metal | AFM-2 | 1.001 | –, 2.676 |
| $Cs_2SnMnCl_6$ | 0.71 | 0.000 | Metal | AFM-2 | 0.999 | –, 4.526 |
| $Cs_2SnFeCl_6$ | 0.71 | 0.000 | Metal | AFM-2 | 1.003 | –, 3.591 |
| $Cs_2SnNiCl_6$ | 0.7 | 0.032 | Metal | AFM-2 | 1.001 | –, 1.489 |
| $Cs_2HgCrCl_6$ | 0.69 | 0.013 | Metal | FM | 1.000 | –, 3.438 |
| $Cs_2HgMnCl_6$ | 0.69 | 0.000 | Insulator | AFM-1 | 1.019 | –, 4.491 |
| $Cs_2HgCoCl_6$ | 0.68 | 0.000 | Metal | AFM-2 | 0.997 | –, 2.520 |
| $Cs_2CdTiCl_6$ | 0.69 | 0.023 | Insulator | AFM-1 | 1.002 | –, 1.622 |
| $Cs_2CdVCl_6$ | 0.67 | 0.035 | Metal | FM | 1.000 | –, 2.687 |
| $Cs_2CdCrCl_6$ | 0.67 | 0.000 | Metal | FM | 0.990 | –, 3.701 |
| $Cs_2CdMnCl_6$ | 0.68 | 0.000 | Insulator | AFM-3 | 1.000 | –, 4.533 |
| $Cs_2SrTiCl_6$ | 0.71 | 0.000 | Metal | AFM-1 | 1.005 | –, 1.635 |
| $Cs_2SrVCl_6$ | 0.71 | 0.018 | Metal | FM | 1.000 | –, 2.668 |
| $Cs_2SrCrCl_6$ | 0.71 | 0.014 | Metal | AFM-1 | 1.054 | –, 3.731 |
| $Cs_2SrMnCl_6$ | 0.71 | 0.001 | Metal | AFM-3 | 1.000 | –, 4.551 |
| $Cs_2MgTiCl_6$ | 0.6 | 0.020 | Metal | FM | 1.005 | –, 1.657 |
| $Cs_2MgVCl_6$ | 0.56 | 0.048 | Metal | FM | 1.000 | –, 2.684 |
| $Cs_2MgCrCl_6$ | 0.57 | 0.013 | Metal | FM | 1.045 | –, 3.739 |
| $Cs_2MgMnCl_6$ | 0.59 | 0.001 | Insulator | AFM-3 | 1.000 | –, 4.558 |
| $Cs_2MgFeCl_6$ | 0.55 | 0.008 | Metal | FM | 1.001 | –, 3.622 |
| $Cs_2ZnTiCl_6$ | 0.61 | 0.044 | Metal | AFM-3 | 0.996 | –, 1.635 |
| $Cs_2ZnCrCl_6$ | 0.58 | 0.006 | Metal | FM | 1.011 | –, 3.731 |
| $Cs_2ZnMnCl_6$ | 0.6 | 0.013 | Insulator | AFM-3 | 1.001 | –, 4.541 |
| $Cs_2ZnFeCl_6$ | 0.57 | 0.007 | Metal | AFM-1 | 1.003 | –, 3.599 |
| $Cs_2ZnCoCl_6$ | 0.54 | 0.019 | Metal | AFM-1 | 0.993 | –, 2.593 |
| $Cs_2GeVCl_6$ | 0.57 | 0.000 | Metal | AFM-2 | 1.000 | –, 2.680 |
| $Cs_2GeCoCl_6$ | 0.53 | 0.000 | Metal | AFM-2 | 0.998 | –, 2.543 |

| $A_2BB'Cl_6$ | $\tau$ | $\Delta H_{hull}$ | **Metal / Insulator (Ground state)** | **Calculated magnetic ground state** | **c/a** | **Calculated magnetic moments, B/B′ $\in$ 3d$^{1-9}$** |
|---|---|---|---|---|---|---|
| $Cs_2TiMnCl_6$ | 0.65 | 0.000 | Metal | AFM-1 | 1.000 | 1.657, 4.545 |
| $Cs_2TiVCl_6$ | 0.64 | 0.042 | Metal | FM | 1.000 | 1.654, 2.670 |
| $Cs_2VMnCl_6$ | 0.62 | 0.020 | Metal | FM | 1.000 | 2.696, 4.549 |
| $Cs_2VCrCl_6$ | 0.61 | 0.038 | Metal | AFM-3 | 1.062 | 2.715, 3.699 |
| $Cs_2CrCoCl_6$ | 0.58 | 0.001 | Metal | AFM-3 | 1.054 | 3.759, 2.673 |
| $Cs_2CrFeCl_6$ | 0.6 | 0.000 | Metal | FM | 1.031 | 3.772, 3.598 |
| $Cs_2CrMnCl_6$ | 0.63 | 0.000 | Metal | FM | 1.038 | 3.782, 4.518 |
| $Cs_2MnCoCl_6$ | 0.6 | 0.000 | Metal | AFM-3 | 1.010 | 4.563, 2.635 |
| $Cs_2MnFeCl_6$ | 0.62 | 0.000 | Metal | AFM-4 | 0.991 | 4.560, 3.652 |
| $Cs_2FeCoCl_6$ | 0.57 | 0.011 | Metal | AFM-3 | 0.966 | 3.908, 2.250 |

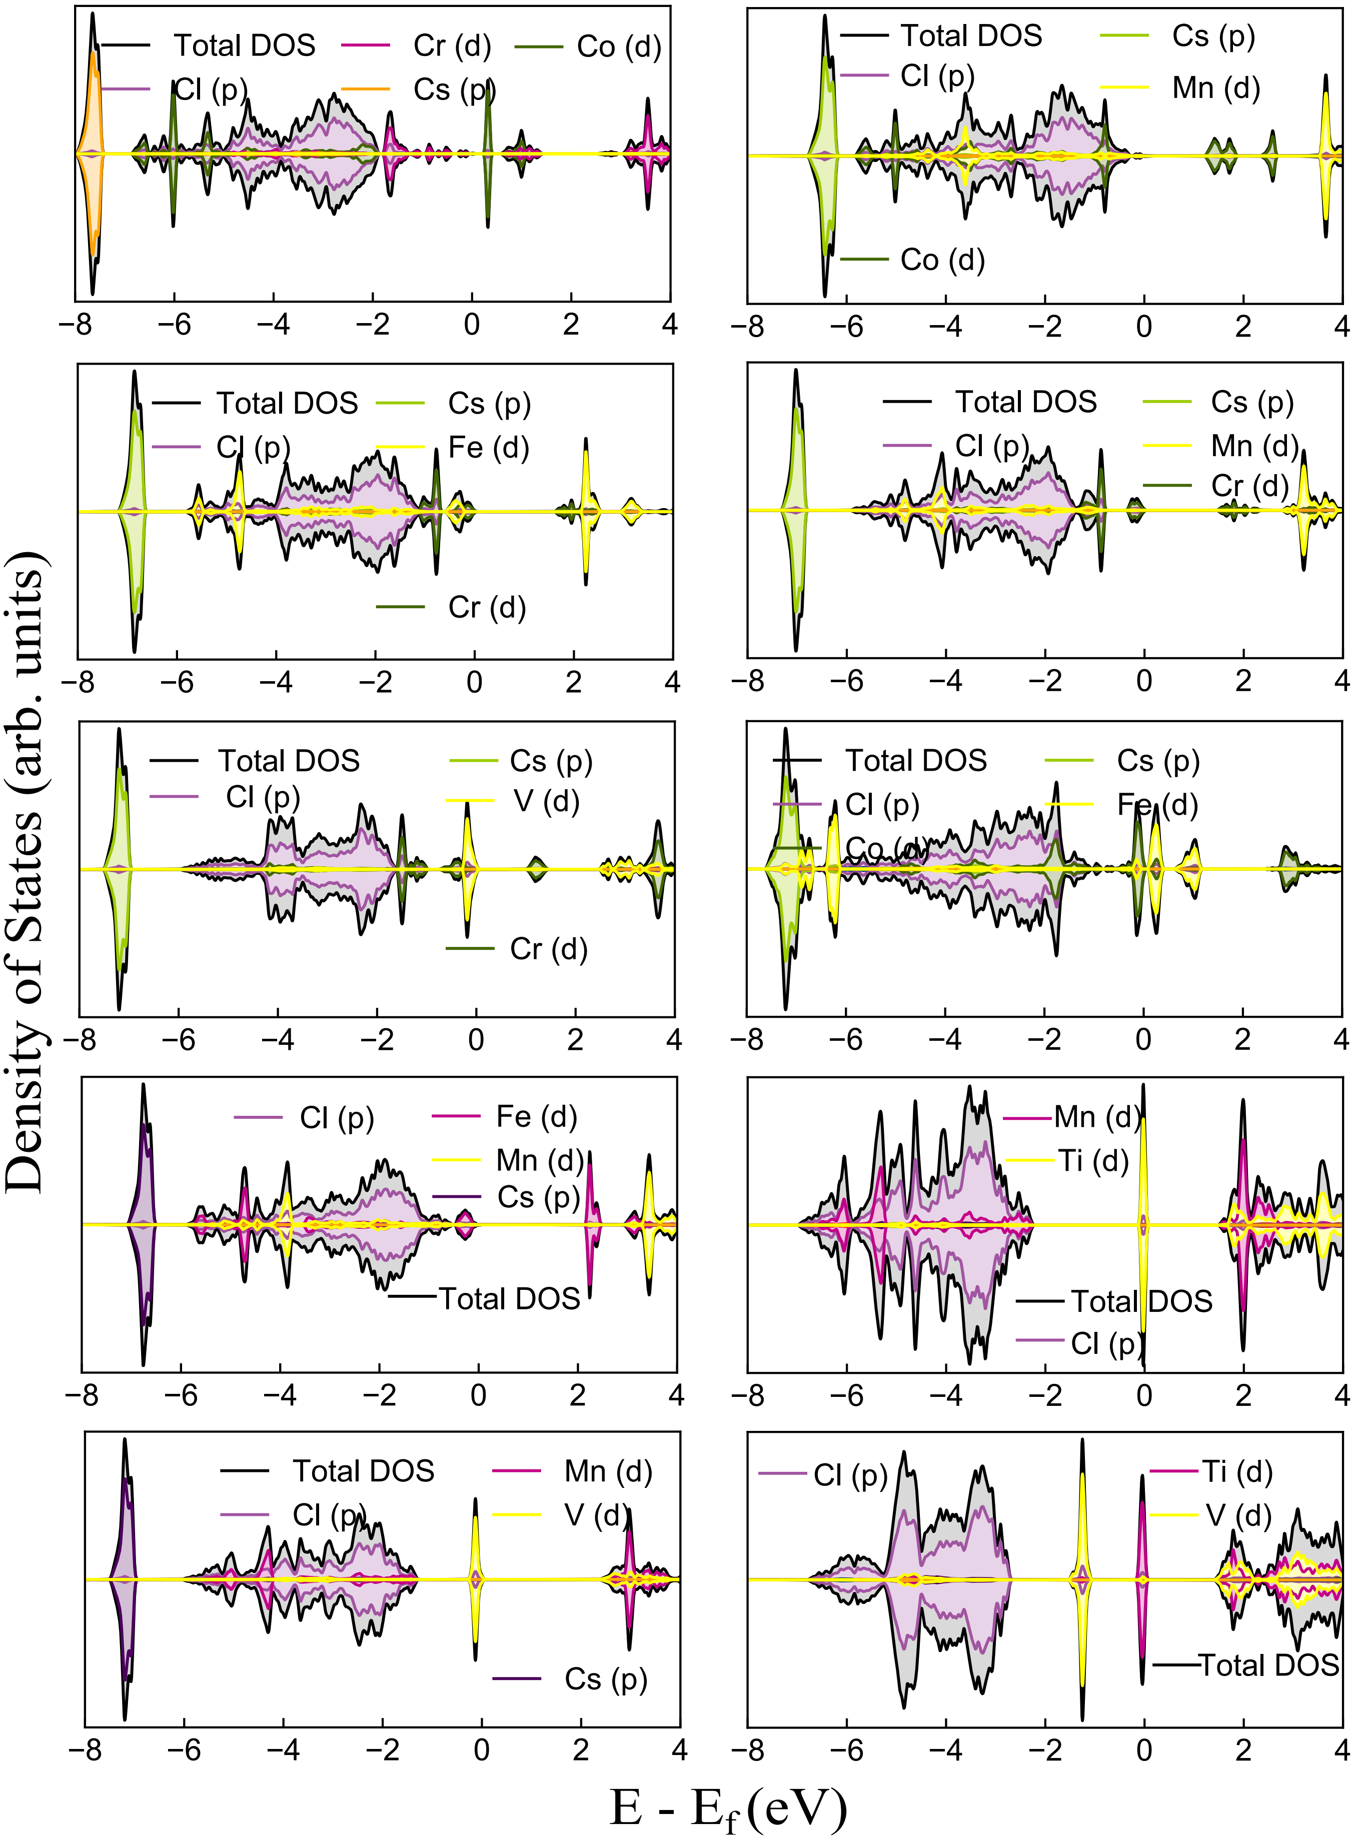


FIG. S1. Density of states for $Cs_2BB'Cl_6$ where both B, $B' \in 3d^{1-9}$.
