# Supplementary material for: Exploring Magnetism of Lead-free Halide Double Perovskites: A High-Throughput First-Principles Study
Source: arXiv:2306.09300 source file (2023-06-15)
Supplement: Supplementary file 2 [file Supplemental_material.pdf]

## Supplementary Information

(Dated: June 15, 2023)

TABLE S1. List of (Column 1) screened  $\text{Cs}_2\text{BB}'\text{Cl}_6$  LFHDPs and corresponding (Column 2) modified tolerance factor,  $\tau$ , (Column 3) distance to convex hull for the cubic ferromagnetic double perovskite phase from previous studies,  $\Delta H_{\text{hull}}$ . The subsequent columns specify the conducting nature, magnetic configuration, and distortion from the cubic phase ( $c/a$ ) respectively of calculated magnetic ground state determined in this work.

| $\text{A}_2\text{BB}'\text{Cl}_6$ | $\tau$ | $\Delta H_{\text{hull}}$ (cubic<br>ferromagnetic<br>phase) | Metal /<br>Insulator<br>(Ground state) | Calculated<br>magnetic<br>ground state | $c/a$ | Calculated<br>magnetic<br>moments,<br>$\text{B/B}' \in 3d^{1-9}$ |
|-----------------------------------|--------|------------------------------------------------------------|----------------------------------------|----------------------------------------|-------|------------------------------------------------------------------|
| $\text{Cs}_2\text{NaTiCl}_6$      | 0.65   | 0.000                                                      | Metal                                  | FM                                     | 0.991 | -, 0.903                                                         |
| $\text{Cs}_2\text{NaVCl}_6$       | 0.64   | 0.000                                                      | Metal                                  | AFM-3                                  | 0.992 | -, 1.918                                                         |
| $\text{Cs}_2\text{NaMnCl}_6$      | 0.64   | 0.000                                                      | Metal                                  | FM                                     | 1.000 | -, 4.035                                                         |
| $\text{Cs}_2\text{NaFeCl}_6$      | 0.64   | 0.000                                                      | Insulator                              | AFM-1                                  | 0.996 | -, 4.053                                                         |
| $\text{Cs}_2\text{NaNiCl}_6$      | 0.62   | 0.025                                                      | Metal                                  | FM                                     | 1.000 | -, 1.000                                                         |
| $\text{Cs}_2\text{KTiCl}_6$       | 0.71   | 0.000                                                      | Metal                                  | FM                                     | 1.002 | -, 0.894                                                         |
| $\text{Cs}_2\text{KVC}_6$         | 0.71   | 0.000                                                      | Metal                                  | FM                                     | 1.010 | -, 1.982                                                         |
| $\text{Cs}_2\text{KCrCl}_6$       | 0.71   | 0.000                                                      | Insulator                              | AFM-1                                  | 1.000 | -, 2.995                                                         |
| $\text{Cs}_2\text{KMnCl}_6$       | 0.71   | 0.000                                                      | Metal                                  | AFM-1                                  | 1.049 | -, 4.014                                                         |
| $\text{Cs}_2\text{KFeCl}_6$       | 0.71   | 0.009                                                      | Insulator                              | AFM-1                                  | 0.996 | -, 4.004                                                         |
| $\text{Cs}_2\text{KNiCl}_6$       | 0.71   | 0.028                                                      | Metal                                  | AFM-1                                  | 1.044 | -, 1.014                                                         |
| $\text{Cs}_2\text{AgMnCl}_6$      | 0.69   | 0.031                                                      | Metal                                  | FM                                     | 1.000 | -, 4.001                                                         |
| $\text{Cs}_2\text{AgNiCl}_6$      | 0.67   | 0.000                                                      | Metal                                  | FM                                     | 1.025 | -, 1.276                                                         |
| $\text{Cs}_2\text{AgTiCl}_6$      | 0.69   | 0.000                                                      | Metal                                  | AFM-1                                  | 0.998 | -, 0.909                                                         |
| $\text{Cs}_2\text{AgFeCl}_6$      | 0.69   | 0.000                                                      | Insulator                              | AFM-1                                  | 0.983 | -, 3.974                                                         |
| $\text{Cs}_2\text{AgVCl}_6$       | 0.68   | 0.000                                                      | Metal                                  | AFM-1                                  | 0.997 | -, 1.951                                                         |
| $\text{Cs}_2\text{AgCoCl}_6$      | 0.68   | 0.000                                                      | Metal                                  | AFM-3                                  | 0.990 | -, 2.501                                                         |
| $\text{Cs}_2\text{AuVCl}_6$       | 0.71   | 0.000                                                      | Insulator                              | FM                                     | 0.896 | -, 2.021                                                         |
| $\text{Cs}_2\text{AuCrCl}_6$      | 0.71   | 0.000                                                      | Metal                                  | AFM-1                                  | 0.926 | -, 3.214                                                         |
| $\text{Cs}_2\text{AuMnCl}_6$      | 0.71   | 0.000                                                      | Metal                                  | FM                                     | 1.000 | -, 4.349                                                         |
| $\text{Cs}_2\text{AuFeCl}_6$      | 0.71   | 0.000                                                      | Insulator                              | AFM-1                                  | 0.934 | -, 3.887                                                         |
| $\text{Cs}_2\text{AuCoCl}_6$      | 0.71   | 0.000                                                      | Metal                                  | AFM-1                                  | 1.105 | -, 2.368                                                         |
| $\text{Cs}_2\text{AuNiCl}_6$      | 0.71   | 0.009                                                      | Metal                                  | FM                                     | 1.098 | -, 1.265                                                         |
| $\text{Cs}_2\text{CaTiCl}_6$      | 0.7    | 0.000                                                      | Metal                                  | FM                                     | 1.004 | -, 1.638                                                         |
| $\text{Cs}_2\text{CaVCl}_6$       | 0.68   | 0.000                                                      | Insulator                              | AFM-3                                  | 1.001 | -, 2.671                                                         |
| $\text{Cs}_2\text{CaCrCl}_6$      | 0.69   | 0.000                                                      | Metal                                  | AFM-1                                  | 1.052 | -, 3.733                                                         |
| $\text{Cs}_2\text{CaMnCl}_6$      | 0.69   | 0.000                                                      | Metal                                  | AFM-3                                  | 1.000 | -, 4.557                                                         |
| $\text{Cs}_2\text{SnVCl}_6$       | 0.71   | 0.039                                                      | Metal                                  | AFM-2                                  | 1.001 | -, 2.676                                                         |
| $\text{Cs}_2\text{SnMnCl}_6$      | 0.71   | 0.000                                                      | Metal                                  | AFM-2                                  | 0.999 | -, 4.526                                                         |
| $\text{Cs}_2\text{SnFeCl}_6$      | 0.71   | 0.000                                                      | Metal                                  | AFM-2                                  | 1.003 | -, 3.591                                                         |
| $\text{Cs}_2\text{SnNiCl}_6$      | 0.7    | 0.032                                                      | Metal                                  | AFM-2                                  | 1.001 | -, 1.489                                                         |
| $\text{Cs}_2\text{HgCrCl}_6$      | 0.69   | 0.013                                                      | Metal                                  | FM                                     | 1.000 | -, 3.438                                                         |
| $\text{Cs}_2\text{HgMnCl}_6$      | 0.69   | 0.000                                                      | Insulator                              | AFM-1                                  | 1.019 | -, 4.491                                                         |
| $\text{Cs}_2\text{HgCoCl}_6$      | 0.68   | 0.000                                                      | Metal                                  | AFM-2                                  | 0.997 | -, 2.520                                                         |
| $\text{Cs}_2\text{CdTiCl}_6$      | 0.69   | 0.023                                                      | Insulator                              | AFM-1                                  | 1.002 | -, 1.622                                                         |
| $\text{Cs}_2\text{CdVCl}_6$       | 0.67   | 0.035                                                      | Metal                                  | FM                                     | 1.000 | -, 2.687                                                         |
| $\text{Cs}_2\text{CdCrCl}_6$      | 0.67   | 0.000                                                      | Metal                                  | FM                                     | 0.990 | -, 3.701                                                         |
| $\text{Cs}_2\text{CdMnCl}_6$      | 0.68   | 0.000                                                      | Insulator                              | AFM-3                                  | 1.000 | -, 4.533                                                         |
| $\text{Cs}_2\text{SrTiCl}_6$      | 0.71   | 0.000                                                      | Metal                                  | AFM-1                                  | 1.005 | -, 1.635                                                         |
| $\text{Cs}_2\text{SrVCl}_6$       | 0.71   | 0.018                                                      | Metal                                  | FM                                     | 1.000 | -, 2.668                                                         |
| $\text{Cs}_2\text{SrCrCl}_6$      | 0.71   | 0.014                                                      | Metal                                  | AFM-1                                  | 1.054 | -, 3.731                                                         |
| $\text{Cs}_2\text{SrMnCl}_6$      | 0.71   | 0.001                                                      | Metal                                  | AFM-3                                  | 1.000 | -, 4.551                                                         |
| $\text{Cs}_2\text{MgTiCl}_6$      | 0.6    | 0.020                                                      | Metal                                  | FM                                     | 1.005 | -, 1.657                                                         |
| $\text{Cs}_2\text{MgVCl}_6$       | 0.56   | 0.048                                                      | Metal                                  | FM                                     | 1.000 | -, 2.684                                                         |
| $\text{Cs}_2\text{MgCrCl}_6$      | 0.57   | 0.013                                                      | Metal                                  | FM                                     | 1.045 | -, 3.739                                                         |
| $\text{Cs}_2\text{MgMnCl}_6$      | 0.59   | 0.001                                                      | Insulator                              | AFM-3                                  | 1.000 | -, 4.558                                                         |
| $\text{Cs}_2\text{MgFeCl}_6$      | 0.55   | 0.008                                                      | Metal                                  | FM                                     | 1.001 | -, 3.622                                                         |
| $\text{Cs}_2\text{ZnTiCl}_6$      | 0.61   | 0.044                                                      | Metal                                  | AFM-3                                  | 0.996 | -, 1.635                                                         |
| $\text{Cs}_2\text{ZnCrCl}_6$      | 0.58   | 0.006                                                      | Metal                                  | FM                                     | 1.011 | -, 3.731                                                         |
| $\text{Cs}_2\text{ZnMnCl}_6$      | 0.6    | 0.013                                                      | Insulator                              | AFM-3                                  | 1.001 | -, 4.541                                                         |
| $\text{Cs}_2\text{ZnFeCl}_6$      | 0.57   | 0.007                                                      | Metal                                  | AFM-1                                  | 1.003 | -, 3.599                                                         |
| $\text{Cs}_2\text{ZnCoCl}_6$      | 0.54   | 0.019                                                      | Metal                                  | AFM-1                                  | 0.993 | -, 2.593                                                         |
| $\text{Cs}_2\text{GeVCl}_6$       | 0.57   | 0.000                                                      | Metal                                  | AFM-2                                  | 1.000 | -, 2.680                                                         |
| $\text{Cs}_2\text{GeCoCl}_6$      | 0.53   | 0.000                                                      | Metal                                  | AFM-2                                  | 0.998 | -, 2.543                                                         |

| $A_2BB'Cl_6$   | $\tau$ | $\Delta H_{\text{hull}}$ | Metal /<br>Insulator<br>(Ground state) | Calculated<br>magnetic<br>ground state | c/a   | Calculated<br>magnetic<br>moments,<br>$B/B' \in 3d^{1-9}$ |
|----------------|--------|--------------------------|----------------------------------------|----------------------------------------|-------|-----------------------------------------------------------|
| $Cs_2TiMnCl_6$ | 0.65   | 0.000                    | Metal                                  | AFM-1                                  | 1.000 | 1.657, 4.545                                              |
| $Cs_2TiVCl_6$  | 0.64   | 0.042                    | Metal                                  | FM                                     | 1.000 | 1.654, 2.670                                              |
| $Cs_2VMnCl_6$  | 0.62   | 0.020                    | Metal                                  | FM                                     | 1.000 | 2.696, 4.549                                              |
| $Cs_2VCrCl_6$  | 0.61   | 0.038                    | Metal                                  | AFM-3                                  | 1.062 | 2.715, 3.699                                              |
| $Cs_2CrCoCl_6$ | 0.58   | 0.001                    | Metal                                  | AFM-3                                  | 1.054 | 3.759, 2.673                                              |
| $Cs_2CrFeCl_6$ | 0.6    | 0.000                    | Metal                                  | FM                                     | 1.031 | 3.772, 3.598                                              |
| $Cs_2CrMnCl_6$ | 0.63   | 0.000                    | Metal                                  | FM                                     | 1.038 | 3.782, 4.518                                              |
| $Cs_2MnCoCl_6$ | 0.6    | 0.000                    | Metal                                  | AFM-3                                  | 1.010 | 4.563, 2.635                                              |
| $Cs_2MnFeCl_6$ | 0.62   | 0.000                    | Metal                                  | AFM-4                                  | 0.991 | 4.560, 3.652                                              |
| $Cs_2FeCoCl_6$ | 0.57   | 0.011                    | Metal                                  | AFM-3                                  | 0.966 | 3.908, 2.250                                              |

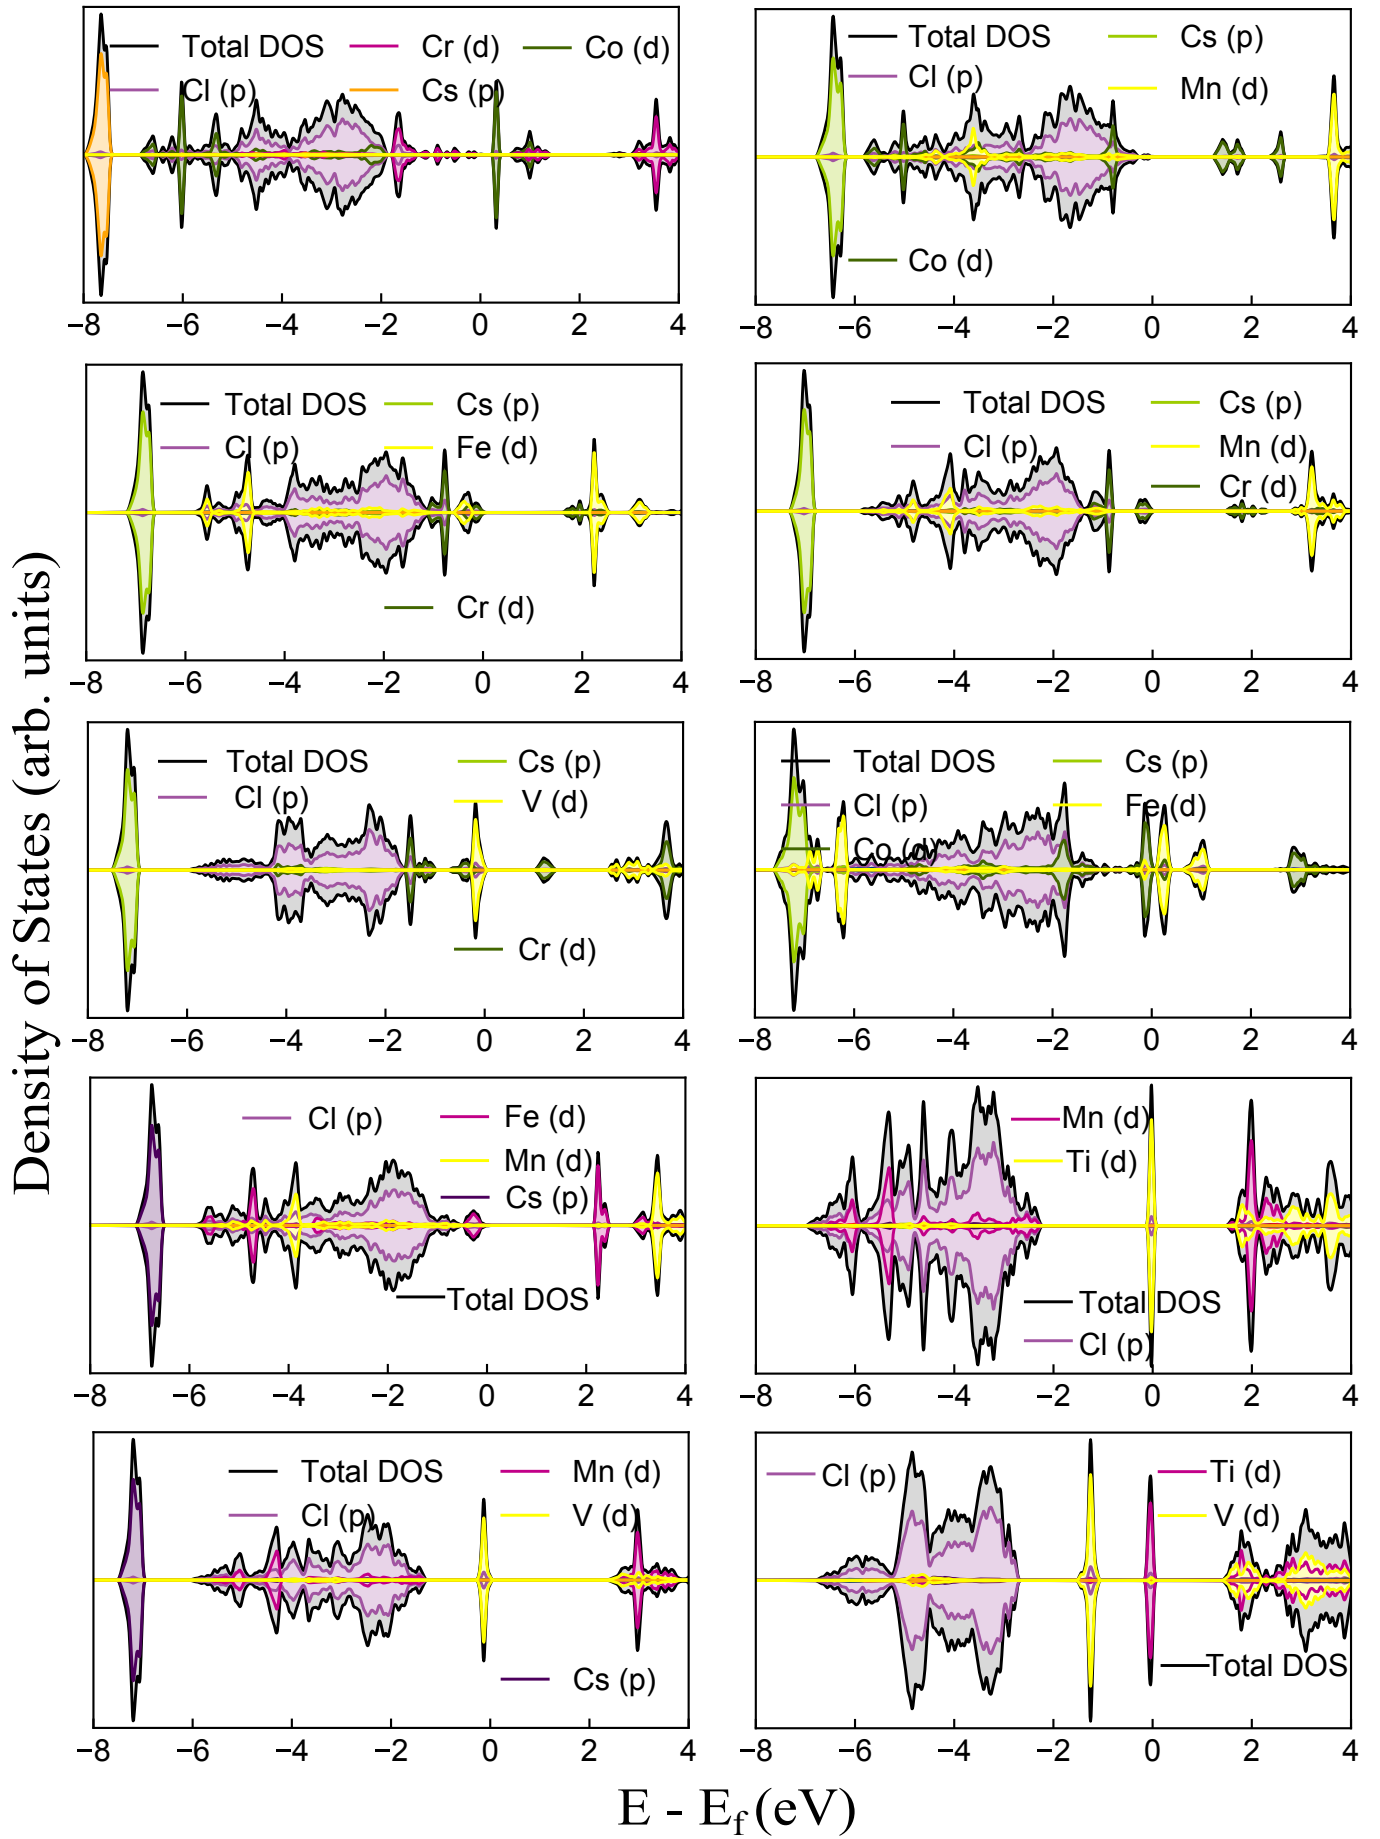

FIG. S1. Density of states for  $\text{Cs}_2\text{BB}'\text{Cl}_6$  where both  $\text{B}, \text{B}' \in 3d^{1-9}$ .
